# Supplementary material for: Unsupervised Visual Attribute Transfer with Reconfigurable Generative Adversarial Networks
Source: arXiv:1707.09798 source file (2017-07-31)
Supplement: Supplementary file 1 [file appendix.tex]

\section{Implementation}

The implementation details of CrisprGAN is summarized in Table \ref{tab:imple}.

\begin{table}[b]
  \centering
  \caption{Network Architectures}   
  \label{tab:imple}
  \begin{tabular}{|l|l|l|}
  \hline
Encoder                                                                                                        & Generator (f=3)                                                                                                  & Discriminator                       \\ \hline
Input 128x128 Color Image                                                                                      & \begin{tabular}[c]{@{}l@{}}Input z: 32x32x256\\ Input f: 32x32x100 (fx100)\\ Concatenate: 32x32x526\end{tabular} & Input 128x128 Color Image           \\ \hline
7x7 Conv, 64 ReLU, BatchNorm                                                                                   & 7x7 Conv, 256 ReLU, BatchNorm                                                                                    & 4x4 Conv, 64 LeakyReLU, BatchNorm   \\ \hline
3x3 Conv, 128 ReLU, BatchNorm                                                                                  & \begin{tabular}[c]{@{}l@{}}{[}Residual{]}\\ 3x3 Conv, 256 ReLU, BatchNorm, \\ 3x3 Conv, BatchNorm\end{tabular}   & 4x4 Conv, 128 LeakyReLU, BatchNorm  \\ \hline
3x3 Conv, 256 ReLU, BatchNorm                                                                                  & \begin{tabular}[c]{@{}l@{}}{[}Residual{]}\\ 3x3 Conv, 256 ReLU, BatchNorm, \\ 3x3 Conv, BatchNorm\end{tabular}   & 4x4 Conv, 256 LeakyReLU, BatchNorm  \\ \hline
\begin{tabular}[c]{@{}l@{}}{[}Residual{]}\\ 3x3 Conv, 256 ReLU, BatchNorm, \\ 3x3 Conv, BatchNorm\end{tabular} & 3x3 Deconv, 128 ReLU, BatchNorm                                                                                  & 4x4 Conv, 512 LeakyReLU, BatchNorm  \\ \hline
                                                                                                               & 3x3 Deconv, 64 ReLU, BatchNorm                                                                                   & 4x4 Conv, 1024 LeakyReLU, BatchNorm \\ \hline
                                                                                                               & 7x7 Conv                                                                                                         & 4x4 Conv                            \\ \hline
                                                                 
  \end{tabular}
\end{table}
